# Supplementary material for: Private Synthetic Data with Hierarchical Structure
Source: arXiv:2206.05942 source file (2022-06-13)
Supplement: Supplementary file 1 [file hpd_derivation.tex]

\subsection{Derivation of query functions in \hpd}\label{appx:hpd_deriv}

\tl{needs to be reworked a bit}

Starting with Definition normalized query and given some synthetic dataset $\hat{D}$ sampled from the distribution $P_\theta$ (parametrized by the parameters $\theta$ of our neural network $F$), we then have that
\begin{equation}\label{eq:norm_query_expectation}
    q_{\phi_1, \phi_2}(P_\theta) 
    = \mathbb{E}_{\hat{D} \sim P_{\theta}} \sbrack{q_{\phi_1, \phi_2}(\hat{D})}
    = \frac{\mathbb{E}_{\hat{D} \sim P_{\theta}} \sbrack{\sum_{x \in \hat{D}} \phi_1(x)}}{\mathbb{E}_{\hat{D} \sim P_{\theta}} \sbrack{\sum_{x \in \hat{D}} \phi_2(x)}}
\end{equation}

Next, we derive the general form of normalized queries \fixed and \generative. In this case, each synthetic dataset sampled from $P_{\textrm{hier}}$ can be written as $\hat{D} = \bigcup_{k=1}^{B} \hat{D}_k$ where each partition $D_k$ is sampled from the product distributions parametrized by the $k^{th}$ row in $F$. Therefore, given some predicate function $\phi = \mathbbm{1}\cc{x \in C}$, we can write
\begin{align*}
    \mathbb{E}_{D \sim P_{F}} \sbrack{\sum_{x \in D} \phi(x)}
    &= \sum_{k=1}^{B} \mathbb{E}_{D_k \sim P_{F_k}} \sbrack{\sum_{x \in D_k} \phi(x)} \\
    &= \sum_{k=1}^{B} \mathbb{E}_{D_k \sim P_{F_k}} \sbrack{\abs{D_k} \mathbb{E} \sbrack{\phi(x) \middle| D_k}} \\
    &= \sum_{k=1}^{B} \mathbb{E}_{D_k \sim P_{F_k}} \sbrack{\abs{D_k} P\pp{x \in C \middle| D_k}}
\end{align*}

For the queries we consider in Section \ref{sec:queries}, we have that $\phi_2 = 1$ (i.e., counts the total number of groups/individuals represented in each sample $D_k$). Therefore, we can rewrite Equation \ref{eq:norm_query_expectation} as
\begin{equation}\label{eq:norm_query_hgem}
    q_{\phi}(P_F) = \frac
    {\sum_{k=1}^{B} \mathbb{E}_{D_k \sim P_{F_k}} \sbrack{\abs{D_k} P\pp{x \in C \middle| D_k}}}
    {\sum_{k=1}^{B} \mathbb{E}_{D_k \sim P_{F_k}} \sbrack{\abs{D_k}}
    }
\end{equation}

To write \textit{individual-level} queries as Equation \ref{eq:norm_query_hgem}, we represent each sample from $F_k$ as a collection of individuals $D_K \in \gY$ (as described in Section \ref{sec:queries} such that $\phi$ is an indicator function. On the other hand for \textit{group-level} queries, we represent each sample as belonging to $\gX$, meaning that $D_k \in \gX$ represents a single group (and the individuals within that group). In this particular case, we have that $\abs{D_k} = 1$, reducing Equation \ref{eq:norm_query_hgem} to
\begin{equation*}
    q_{\phi}(P_F) = \frac{1}{B}
    \sum_{k=1}^{B} \mathbb{E}_{D_k \sim P_{F_k}} \sbrack{P\pp{x \in C \middle| D_k}}
\end{equation*}

Given that we output a product distribution $F_G$ for \textit{group-level} attributes and separate distributions $F_I$ for each individual belonging to a group, we can conveniently switch between data domains $\gX$ and $\gY$ such that we can answer both query types using our set of product distributions. As a result, \fixed and \generative can jointly optimize over both query types as long as $P\pp{x \in C \middle| D_k}$ can be written down as some function that is differentiable w.r.t. the parameters of $F$.
